# Supplementary material for: Evaluating the Diversity and Quality of LLM Generated Content
Source: arXiv:2504.12522 source file (2026-02-26)
Supplement: Supplementary file 1 [file appendix_correctness_benchmarks.tex]

\subsection{Model Correctness Benchmarks}
\newcolumntype{Y}{>{\centering\arraybackslash}X}

% \begin{table*}[!h]
%     \centering
%     \footnotesize
%     \setlength{\tabcolsep}{2pt}
%     \arrayrulecolor{blue} % Set table borders to blue
%     \begin{tabularx}{\textwidth}{c|*{1}{Y}|*{1}{Y}}
%     \toprule

%        & \multicolumn{1}{c|}{\textbf{Base Model}} & \multicolumn{1}{c}{\textbf{Instruction-Tuned}} \\
%     \midrule
%     % \textbf{Model} & \textbf{Coh.} & \textbf{Sem.} & \textbf{Syn.} & \textbf{Lex.} & \textbf{ $\Delta$ Coh.} & \textbf{ $\Delta$ Sem.} & \textbf{ $\Delta$ Syn.} & \textbf{ $\Delta$ Lex.} \\
%     \toprule
%     \textsc{CodeLlama-7B}  & 33.5 & 34.8 \\
%     \textsc{CodeLlama-34B} & 48.8 & 41.5 \\
%     \textsc{CodeLlama-70B} & 53.0 & 67.8 \\
%     \midrule
%     \textsc{Meta-Llama-3-8B} & 37.2 & 60.4 \\
%     \textsc{Meta-Llama-3-70B} & 58.5 & 81.7 \\
%     \midrule
%     \textsc{Meta-Llama-3.1-8B} & - & 72.6 \\
%     \textsc{Meta-Llama-3.1-70B} & - & 80.5 \\
%     \bottomrule

%     \end{tabularx}
%     \caption{\reb{\label{tab:base_vs_instruct_humaneval} Pass@1 performance of all tested models on HumanEval benchmark (0-Shot).}}
% \end{table*}

\begin{table}[h]
  \center
   \setlength{\tabcolsep}{3pt}
   \arrayrulecolor{blue} % Set table borders to blue
  \begin{tabular}{lr|cc} 
  \toprule
  \textbf{Model} &\multicolumn{1}{c}{\textbf{Size}}& \multicolumn{2}{c}{Code Generation Benchmarks} \\  
  && \textbf{HumanEval} & \textbf{MBPP} \\ 
  \midrule
  \multirow{3}{*}{\codellama} 
  & 7B  & 33.5 & 41.4 \\
  &34B  & 48.8 & 55.0 \\
  &70B  & 53.0 & 62.4 \\
  \midrule
  \multirow{3}{*}{\codellamainst} 
  &7B  & 34.8 & 44.4 \\
  &34B  & 41.5 & 57.0 \\
  &70B  & 67.8 & 62.2 \\
  \midrule
  \multirow{3}{*}{\codellamapy} 
  &7B  & 38.4 & 47.6 \\
  &34B  & 53.7 & 56.2 \\
  &70B  & 57.3 & 65.6 \\
  \midrule
  \midrule
  \multirow{2}{*}{\llamathree}
  &8B  & 37.2 & - \\
  &70B  & 58.5 & - \\
  \midrule
  \multirow{2}{*}{\llamathreeone}
  &8B  & 8.5 & 47.6 \\
  &70B  & - & 66.2 \\
  \midrule
  % \multirow{1}{*}{Mistral}
  % &7B  & 30.5  & 47.5 \\
  % \multirow{1}{*}{Mixtral}
  % &8$\times$22B  & 45.1 & 71.2 \\
  % \cmidrule[1.3pt]{1-4} % Adjusted thicker line
  \multirow{2}{*}{\llamathreeinst} 
  &8B  & 60.4 & 70.6 \\
  &70B  & 81.7 & 82.5 \\
  \midrule
  \multirow{2}{*}{\llamathreeoneinst} 
  &8B  & 72.6 & 72.8 \\
  &70B  & 80.5 & 86.0 \\
  % \midrule
  % \multirow{1}{*}{Mistral-Instruct}
  % &7B  & 40.2 & 49.5 \\
  % \multirow{1}{*}{Mixtral-Instruct}
  % &8$\times$22B  & 75.6 & 78.6 \\
  \midrule
  \midrule
  \multirow{3}{*}{Qwen2.5-Coder} 
  & 7B  & 61.6 & 76.9 \\
  &14B  & 64.0 & 81.0 \\
  &32B  & 65.9 & 83.0 \\
  \midrule
  \multirow{3}{*}{Qwen2.5-Coder-Instruct} 
  &7B  & 88.4 & 83.5 \\
  &14B  & 89.6 & 86.2 \\
  &32B  & 92.7 & 90.2 \\
  \midrule
  \midrule
  \multirow{1}{*}{\texttt{code-davinci-002}}
  &  & 47.0 & 58.10 \\
  \multirow{1}{*}{\texttt{gpt-3.5-turbo-0125}}
  &  & 48.1 & - \\
  \multirow{1}{*}{\texttt{gpt-3.5-turbo-instruct}}
  &  & 68.0 & 82.0 \\
  \multirow{1}{*}{\texttt{gpt-4o-mini}}
  &  & 87.2 & - \\
  \cmidrule[1.3pt]{1-4} % Adjusted thicker line
  \multirow{1}{*}{Claude 3 Sonnet}
  &  & 73.0 & 79.4 \\
  \multirow{1}{*}{Claude 3 Haiku}
  &  & 75.9 & 80.4 \\
  \bottomrule
  \end{tabular}
  \caption{\reb{\textbf{Pass@1 scores on HumanEval and MBPP.} Results for the models as provided by~\cite{codellama-2023} (\codellama), \cite{llama3-2024} (\llamathree, \llamathreeone, Mistral, \texttt{gpt-3.5-turbo-instruct}), \cite{qwen} (Qwen2.5-Coder), \cite{zheng2023survey} (\texttt{code-davinci-002}), \cite{achiam2023gpt} (\texttt{gpt-3.5-turbo-0125}, \texttt{gpt-4o-mini}), and \cite{anthropic2024claude3} (Claude 3).}}
\label{tab:correctness}
\end{table}
