# Supplementary material for: Evaluating the Diversity and Quality of LLM Generated Content
Source: arXiv:2504.12522 source file (2026-02-26)
Supplement: Supplementary file 2 [file appendix_correlation_analysis.tex]

\subsection{Additional Discussion and Analysis on \textsc{CodeBertScore}}
\label{subsec:correlation_analysis}

In \Cref{subsec:reflecting_semantics}, we evaluate the correlation between pairs of diversity metrics $m_1$ and $m_2$; to summarize these results, we report the Spearman and Kendall's Tau Rank Correlation coefficients of the values $\text{Div}_{m_1}(P_i)$ and $\text{Div}_{m_2}(P_i)$ aggregated across all sets of generations $P_i$ over all problem descriptions and all models.

\textbf{Existing diversity metrics fail to reflect execution semantics.} We report the Spearman and Kendall's Tau rank correlation coefficient matrices for diversity metrics in \Cref{fig:combined-corr}. \reb{Our purpose is to motivate that diversity in program execution struggles to be captured by (and may even be negatively correlated with) lexical and neural diversity metrics. This is in line with prior work demonstrating that lexical and neural similarity metrics, at best, correlate relatively weakly with \textit{functional correctness} \citep{hendrycksapps2021, codebertscore2023, icescore}, \textit{however now for diversity}.} We find that neural, lexical, and syntactic diversity fail to reflect semantic diversity based on executions accurately. All are negatively correlated.
Additionally, lexical, syntactic, and neural diversity are all inter-correlated to varying degrees. Given that neural metrics fail to reflect execution semantics, they did not offer insight into other forms of diversity for our task, so we omit them from subsequent experiments. In \Cref{subsec:effect_of_instr_tuning}, we find a tradeoff in semantic diversity and lexical/syntactic diversity with instruction tuning. Given the large amount base and instruct models under consideration, these kinds of phenomena may contribute to the negative correlations. 
%\alex{I will update this paragraph + Try to do more error analyzis, the correlations are all NEGATIVE after using more samples}

\textbf{Program semantics may be more complicated to model than natural language.} Programming is a skill-intensive activity, and often, minor details can greatly impact program behavior. Whereas models can achieve over 90\% accuracy on textual entailment tasks  ~\citep{he2021debertadecodingenhancedbertdisentangled, zhong2022efficientlanguagemodelpretraining}, \textsc{CodeBertScore} and \textsc{ICE-Score} report a moderate correlation with accuracy \citep{codebertscore2023, icescore}. The complex nature of understanding programs combined with diverse and off-distribution generations may contribute to the relationships observed. 

% In \Cref{subsec:correlation_analysis} \alex{Don't forget to include this}, we provide evidence ruling out the short context window of \texttt{512} tokens as a factor in \textsc{CodeBertScore}'s errors. 
% We find weak evidence that off-distribution content may be related to errors. 
Anecdotally, for \textsc{CodeBertScore} we found minor differences like a \texttt{min} instead of a \texttt{max}, and extra comments / unrelated generated code could trigger poor performance. Even though we may identify failure modes with our strict notion of semantics, this may be expected given \textsc{CodeBertScore} is not trained on execution semantics, and examples such as those in \Cref{fig:codebertscores-comparison} code are still related. Our takeaway is that we should not prima facie assume neural models can fully capture true semantic diversity: caution should used when evaluating diversity at scale, especially for programs. 

With regard to the CodeBertScore Classifier metric, we believe that it is possible the metric may breakdown due to numerous reasons. Anyone who has read code can also attest that deeply understanding a program and reasoning about its execution semantics can often be extremely difficult, and \textsc{CodeBertScore} itself does not correlate highly with functional correctness in Python \citep{codebertscore2023}. The challenge of modeling semantics is even more so the case given that our programs contain anonymized function signatures which do not provide any hints on what the program is supposed to do. It is also plausible that errors have other causes: in \Cref{??} we perform a more in-depth error analysis where we rule out the limited context window of \texttt{512} tokens as an error source. Instead we found weak evidence that as the generations were more off-distrubution (as measured by higher perplexity by \textsc{CodeLLama7b-Python}) that the CodeBertScore Classifier metric suffered. 

Given that neural metrics fail to reflect execution semantics on this task, they did not offer us interpretable insight into other forms of diversity for this task. As a result, we omit them from our analysis.
