# Supplementary material for: Evaluating the Diversity and Quality of LLM Generated Content
Source: arXiv:2504.12522 source file (2026-02-26)
Supplement: Supplementary file 3 [file appendix_metrics.tex]

\subsection{Diversity Metrics}
\label{sec:metrics}

\alex{I think we can trim this down aggressively, and put the full details into the appendix. Distinct-N, Syntax, Neural should be fast. I think Semantic we can provide more concrete detail on.} \shuo{I agree. I think putting too much details about lexical, syntactic and neural diversity measures in the main body might even distract the readers from our main contribution.}

Next, we describe the metrics used to measure diversity, focusing specifically on our choice of $\text{Div}_m(P_i)$.

% pairwise distance $m_{\text {dist}}(g, g')$. 

\textbf{Semantic diversity.} To measure the semantic diversity $m_{\text {dist}}(g, g')$, we first specify the validity function $V$ and semantic function $S$ introduced in Section~\ref{sec:formulation}. Specifically, let $T = \{t_1, \ldots, t_M\}$ be a set of specified test cases, $p$ be a generated program that takes in a test case $t_m$ and output the execution result $o_m$. We define the validity function $V$ as identifying if any errors, like \textit{SyntaxError}, \textit{ValueError}, are encountered when executing $g$ on $T$. If no error is triggered, we set $V(g)=1$; otherwise, $V(g)=0$. We define the semantic function $S$ as executing the $g$ on $T$ and outputting the corresponding execution results $\{o_m\}_{m=1}^M$. Intuitively, the semantic function $S$ identifies the semantic meaning of $g$ by its execution results on $T$. Furthermore, for two program $g, g'$ and their corresponding execution results $\{o_m\}_{m=1}^M, \{o'_m\}_{m=1}^M$, we define $S(g)=S(g')$ if $o_m=o'_m, \ \forall m \in \{1, \ldots, M\}$.

For \textbf{Lexical diversity,} we use Expectation-Adjusted Distinct $n$-grams (\textbf{EAD}), an adaptation of the Distinct-N metric that removes bias towards shorter sequence length~\citep{ead-diversity-2022, rlhf-diversity-2023}. The Distinct-N metric~\citep{distinct-n-2016,distinct_n_2019} computes the ratio between the number of \textit{unique} $n$-grams divided by the \textit{total} number of $n$-grams; in our case, we apply this to the combined text of the two generated programs. We tokenize programs using the Parso Tokenizer,\footnote{\url{https://github.com/davidhalter/parso}} which allows tokenization of Python in the presence of syntax errors. We report EAD using $n$-grams of length $n$$=$4.  For our lexical and syntactic diversity metrics, we approximate \Cref{eq:distness_kernel} by randomly sampling 300 pairs with replacement for efficiency.
%\alex{this is sort of repeated in the background section}

\textbf{Syntactic diversity.} We adapt the Distinct-N metric to the Abstract Syntax Tree (\textbf{AST}) of each generated program. To further isolate the syntactic structure of a program (e.g., for-loop instead of recursion) from superficial choices (e.g., variable names), we canonicalize all identifiers and numeric constants in the AST, which we call the \textbf{Canonicalized AST}. We implement the Distinct measure on Canonicalized ASTs for two programs by calculating the ratio of the number of unique subtrees of height $H$ across both programs to the total number of subtrees of height $H$ in both programs, where $H$$=$4. In \Cref{subsec:appendix_diversity}, we provide a figure visually demonstrating a Canoncalized AST for a small Python expression and additional implementation details. 

\textbf{Neural diversity.}  We adapt existing methods of neural diversity metrics  \citep{evaluating-the-evaluation-2021} to our domain by using \textsc{CodeBertScore} \citep{codebertscore2023} \reb{and \textsc{ICE-Score}, an LLM-based code-evaluation tool \citep{icescore}. For \textsc{ICE-Score}, we use \texttt{gpt-4o-2024-11-20} and the functional correctness setting. Since higher scores should indicate higher similarity, we use $1 - \text{Score}(p_j, p_k)$ for distinctness.}
While \textsc{CodeBertScore} and \textsc{ICE-Score} were not intended for evaluating program diversity, we choose them since it either closely resemble models used in the NLP literature to evaluate semantic diversity \citep{evaluating-the-evaluation-2021} or are state-of-the-art in neural code evaluation.

In our analysis, we report this number as the semantic diversity in the context of all samples taken: if a generation does not contain a program, we penalize the model as it does not produce semantically meaningful content. 

\textbf{Coherence.} We additionally report a metric that measures the ``quality'' of generations. We use the term ``coherence'' to describe a well-formed generation with the following properties: (i) contains the definition of the function $f(...)$, (ii) has no syntax errors, (iii) is capable of being run on all test cases without runtime errors, and (iv) prints out any output (as requested by the prompt).
